# Supplementary material for: Statistical screening model for moderately coupled and dense plasmas
Source: arXiv:2007.05243 source file (2020-11-24)
Supplement: Supplementary file 1 [file Supplemental_Material.pdf]

**Supplementary information for**

# Statistical screening model for moderately coupled and dense plasmas

## I. Model Formulation

In this work, we have defined a coefficient

$$\chi^j = \frac{n_e^2 n_{ion}\beta_j + \sum_{j'} n_e n_{atom}^{j'} K_{j'j}}{n_e^2 n_{ion}\beta_j + \sum_{j'} n_e n_{atom,equil}^{j'} K_{j'j}}, \qquad (1)$$

to describe the non-equilibrium feature of plasma-electron distribution around the targeted ion, and then the population density of negative-energy state is given by $n_{atom}^j = \chi^j n_{atom,equil}^j$. Here, $\alpha_j$ and $\beta_j$ are the rate coefficients of electron impact ionization and three-body recombination, $K_{j'j}$ and $K_{jj'}$ are the rate ones of excitation and de-excitation. $n_{atom,equil}^j$ is the population density for an equilibrated system, which can be calculated by Fermi-Dirac statistics within given free-electron density $n_e$, temperature $T_e$ and effective potential $\Phi(r)$. For the targeted ion, $\sum_{j'} n_{atom}^{j'} < \sum_{j'} n_{atom,equil}^{j'}$ and $\chi^j$ can be approximated as

$$\chi^j = \frac{n_e^2 n_{ion}\beta_j}{n_e^2 n_{ion}\beta_j + \sum_{j'} n_e n_{atom,equil}^{j'} K_{j'j}}. \qquad (2)$$

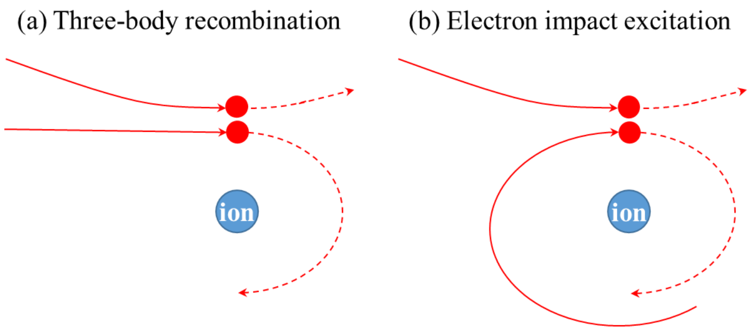


Figure 1 Diagrams of three-body recombination and electron impact excitation from the classical point of view.

From the classical point of view, the density of electrons in phase space, i.e. $f(\boldsymbol{p},\boldsymbol{r})$ with $p^2/2m_e < e\Phi(\boldsymbol{r})$, is introduced to instead of $n_{atom}^j$. For a system in equilibrium, $f(\boldsymbol{p},\boldsymbol{r})$ can be described by Fermi-Dirac or Boltzmann distribution. The probability of collision between two electrons with velocities $\boldsymbol{v}_1'$ and $\boldsymbol{v}_2'$ into velocities $\boldsymbol{v}_1$ and $\boldsymbol{v}_2$ at position $\boldsymbol{r}$ is given by

$$I^{in}(\boldsymbol{v}_1) = \int d\boldsymbol{v}_1' \int d\boldsymbol{v}_2' \int d\boldsymbol{v}_2\, f(\boldsymbol{v}_1') f(\boldsymbol{v}_2') \sigma(\boldsymbol{v}_1',\boldsymbol{v}_2' \to \boldsymbol{v}_1,\boldsymbol{v}_2)\, v. \qquad (3)$$

Here, $\sigma(\boldsymbol{v}_1',\boldsymbol{v}_2' \to \boldsymbol{v}_1,\boldsymbol{v}_2)$ is the scattering cross section and $v$ is the relative velocity between two electrons. It is assumed that the population density for the state with velocity $\boldsymbol{v}_1'$ and $\boldsymbol{v}_2'$ is approximated as $f(\boldsymbol{v}_1')f(\boldsymbol{v}_2')$, i.e. the famous molecular chaos assumption. As shown in figure 1, both three-body recombination and electron impact excitation can produce the negative-energy electron with $\frac{1}{2}m_e v_1^2 < e\Phi(\boldsymbol{r})$. By using Eq. (2), the non-equilibrium coefficient can be expressed as

$$\chi(\boldsymbol{p},\boldsymbol{r}) = \chi(\boldsymbol{v}_1,\boldsymbol{r}) = \frac{I_{recomb}^{in}(\boldsymbol{v}_1)}{I^{in}(\boldsymbol{v}_1)}, \qquad (4)$$

where $I_{recomb}^{in}(\boldsymbol{v_1})$ represents the recombination probability of free electron to recombined bound one with negative energy, and can be expressed as

$$I_{recomb}^{in}(\boldsymbol{v_1}) = \int d\boldsymbol{v_1'} \int d\boldsymbol{v_2'} \int d\boldsymbol{v_2}\, \theta\left(\frac{1}{2}m_e {v_1'}^2 - e\Phi(\boldsymbol{r})\right) f(\boldsymbol{v_1'}) f(\boldsymbol{v_2'}) \sigma(\boldsymbol{v_1'}, \boldsymbol{v_2'} \to \boldsymbol{v_1}, \boldsymbol{v_2})\, v. \qquad (5)$$

Here, $\theta(\frac{1}{2}m_e {v_1'}^2 - e\Phi(\boldsymbol{r}))$ is the step function, which guarantees that the electron $\boldsymbol{v_1'}$ be free.

In order to obtain the non-equilibrium coefficient $\chi(\boldsymbol{p}, \boldsymbol{r})$, two-electron model is used to compute the scattering cross section

$$\sigma(\theta) = \frac{e^4}{m_e^2 v^4 \left[\sin^2\frac{\theta}{2} + \left(\frac{\theta_m}{2}\right)^2\right]^2} \qquad (6)$$

$$\text{with } \theta_m = \frac{2\hbar}{m_e v \lambda_D},$$

in which plasma screening effects is described with Debye-Hückel potential $\frac{1}{r}exp(-r/\lambda_D)$ and screening length $\lambda_D$, $\theta$ is the angle between the initial and final relative velocities of $\boldsymbol{v}'$ and $\boldsymbol{v}$. With the centroid and the relative velocity of the two electrons system defined as

$$\boldsymbol{V_C} = \frac{m_e\boldsymbol{v_1} + m_e\boldsymbol{v_2}}{m_e + m_e} = \frac{1}{2}(\boldsymbol{v_1} + \boldsymbol{v_2}) \qquad (7)$$

and

$$\boldsymbol{v} = \boldsymbol{v_1} - \boldsymbol{v_2}, \qquad (8)$$

the scattering cross section in center of mass system can be expressed as

$$\sigma(\boldsymbol{v_1'}, \boldsymbol{v_2'} \to \boldsymbol{v_1}, \boldsymbol{v_2}) = \sigma(\theta)\frac{\delta(v - v')}{v^2}\delta(\boldsymbol{V_C'} - \boldsymbol{V_C}). \qquad (9)$$

Inserting Boltzmann distribution $f(\boldsymbol{v_1'}) = \Lambda_e exp\,(-\frac{m_e {v_1'}^2}{2k_BT})$ and the equations (9) into equation (3), the total scattering probability can be obtained as

$$I^{in}(\boldsymbol{v_1}) = \int d\boldsymbol{v_1'} \int d\boldsymbol{v_2'} \int d\boldsymbol{v_2}\, \Lambda_e exp\left(-\frac{m_e {v_1'}^2}{2k_BT}\right) \Lambda_e exp\left(-\frac{m_e {v_2'}^2}{2k_BT}\right) \sigma(\boldsymbol{v_1'}, \boldsymbol{v_2'} \to \boldsymbol{v_1}, \boldsymbol{v_2})\, v$$

$$= \int d\boldsymbol{V_C'} \int dv' \int d\boldsymbol{v_2}\, \Lambda_e^2 exp\left(-\frac{m_e {V_C'}^2 + \frac{1}{4}m_e {v'}^2}{k_BT}\right) \sigma(\theta)\frac{\delta(v - v')}{v^2}\delta(\boldsymbol{V_C'} - \boldsymbol{V_C})\, v$$

$$= \Lambda_e^2 \int d\boldsymbol{v_2}\, exp\left(-\frac{m_e V_C^2 + \frac{1}{4}m_e v^2}{k_BT}\right) \frac{4\pi e^4 \lambda_D^2}{\hbar^2 v} \frac{1}{1 + \hbar^2/(m_e v \lambda_D)^2}$$

$$= \Lambda_e^2 exp\left(-\frac{m_e v_1^2}{2k_BT}\right) \int_0^{\pi} 2\pi sin\phi d\phi \int_0^{\infty} v_2^2 dv_2\, exp\left(-\frac{m_e v_2^2}{2k_BT}\right)$$

$$\times \frac{4\pi e^4 \lambda_D^2}{\hbar^2 \sqrt{(cos\phi v_2 - v_1)^2 + (sin\phi v_2)^2}\left(1 + \frac{\hbar^2}{m_e \lambda_D^2[(cos\phi v_2 - v_1)^2 + (sin\phi v_2)^2]}\right)}, \qquad (10)$$

where $\Lambda_e = \sqrt{2\pi\hbar^2/(m_e k_B T)}$. Similarly, the electron recombination probability $I_{recomb}^{in}(\boldsymbol{v_1})$ can be obtained as

$$I_{recomb}^{in}(\boldsymbol{v_1}) = \int d\boldsymbol{V'_C} \int d\boldsymbol{v'} \int d\boldsymbol{v_2}\, \theta\left(m_e V_C'^2 + \frac{1}{4} m_e v'^2 - m_e \boldsymbol{V'_C} \cdot \boldsymbol{v'} - e\Phi(\boldsymbol{r})\right)$$

$$\times \Lambda_e^2 e^{-\frac{1}{k_B T}(m_e V_C'^2 + \frac{1}{4} m_e v'^2)} \sigma(\theta) \frac{\delta(v - v')}{v^2} \delta(\boldsymbol{V'_C} - \boldsymbol{V_C})\, v\,. \quad (11)$$

For simplicity, with the average of the angle between $\boldsymbol{V'_C}$ and $\boldsymbol{v'}$ the step function is approximated to $\theta\left(m_e V_C'^2 + \frac{1}{4} m_e v'^2 - e\Phi(\boldsymbol{r})\right)$. Then, the equation (11) can be reduced to

$$I_{recomb}^{in}(\boldsymbol{v_1}) = \Lambda_e^2 \int d\boldsymbol{v_2}\, \theta\left(m_e V_C^2 + \frac{1}{4} m_e v^2 - e\Phi(\boldsymbol{r})\right) exp\left(-\frac{m_e V_C^2 + \frac{1}{4} m_e v^2}{k_B T}\right) \frac{4\pi e^4 \lambda_D^2}{\hbar^2 v} \frac{1}{1 + \hbar^2/(m_e v \lambda_D)^2}$$

$$= \Lambda_e^2 exp\left(-\frac{m_e v_1^2}{2k_B T}\right) \int_0^{\pi} 2\pi sin\phi d\phi \int_{\sqrt{2\varepsilon_r/m_e}}^{\infty} v_2^2 dv_2\, exp\left(-\frac{m_e v_2^2}{2k_B T}\right)$$

$$\times \frac{4\pi e^4 \lambda_D^2}{\hbar^2 \sqrt{(cos\phi v_2 - v_1)^2 + (sin\phi v_2)^2}\left(1 + \frac{\hbar^2}{m_e \lambda_D^2[(cos\phi v_2 - v_1)^2 + (sin\phi v_2)^2]}\right)}, \quad (12)$$

where $\varepsilon_r = e\Phi(r) - \frac{1}{2} m_e v_1^2$. Inserting the equations (10) and (12) into (4), the non-equilibrium coefficient $\chi(\boldsymbol{p}, \boldsymbol{r})$ can be calculated numerically by

$$\chi(\boldsymbol{p}, \boldsymbol{r}) = \chi(\boldsymbol{v_1}, \boldsymbol{r})$$

$$= \frac{\int_0^{\pi} d\phi \int_{\sqrt{2\varepsilon_r/m_e}}^{\infty} dv_2 \frac{exp\left(-\frac{m_e v_2^2}{2k_B T}\right) sin\phi v_2^2}{\sqrt{(cos\phi v_2 - v_1)^2 + (sin\phi v_2)^2}\left(1 + \frac{\hbar^2}{m_e \lambda_D^2[(cos\phi v_2 - v_1)^2 + (sin\phi v_2)^2]}\right)}}{\int_0^{\pi} d\phi \int_0^{\infty} dv_2 \frac{exp\left(-\frac{m_e v_2^2}{2k_B T}\right) sin\phi v_2^2}{\sqrt{(cos\phi v_2 - v_1)^2 + (sin\phi v_2)^2}\left(1 + \frac{\hbar^2}{m_e \lambda_D^2[(cos\phi v_2 - v_1)^2 + (sin\phi v_2)^2]}\right)}}. \quad (13)$$

For the UNP and hot-dense plasmas studied in this work, the condition of $\hbar^2/(m_e \lambda_D^2 v^2) \ll 1$ is satisfied, and the non-equilibrium coefficient can be further simplified as

$$\chi(\boldsymbol{p}, \boldsymbol{r}) = \frac{\int_0^{\pi} d\phi \int_{\sqrt{2\varepsilon_r/m_e}}^{\infty} dv_2 \frac{exp\left(-\frac{m_e v_2^2}{2k_B T}\right) sin\phi v_2^2}{\sqrt{(cos\phi v_2 - v_1)^2 + (sin\phi v_2)^2}}}{\int_0^{\pi} d\phi \int_0^{\infty} dv_2 \frac{exp\left(-\frac{m_e v_2^2}{2k_B T}\right) sin\phi v_2^2}{\sqrt{(cos\phi v_2 - v_1)^2 + (sin\phi v_2)^2}}} = 2\sqrt{\varepsilon_r/(\pi k_B T)} e^{-\frac{\varepsilon_r}{k_B T}} / Erf\left(\sqrt{\varepsilon_r/(k_B T)}\right). \quad (14)$$

Here $Erf(x)$ is the error function, and $\varepsilon_r = e\Phi(\boldsymbol{r}) - p^2/2m_e$. The equation (14) can also be obtained based on the scattering cross section of hard sphere model,

$$\sigma(\theta) = \frac{R^2}{4}, \quad (15)$$

where *R* is the diameter of particles. It is indicated that $\chi(\boldsymbol{p}, \boldsymbol{r})$ is not sensitive to the scattering model employed.

With $\chi(\boldsymbol{p}, \boldsymbol{r})$ obtained, the negative-energy density distribution function can be calculated with $f_{FD}(\boldsymbol{p}, \boldsymbol{r})\chi(\boldsymbol{p}, \boldsymbol{r})$, and the total plasma-electron density is given by

$$\rho(\boldsymbol{r}) = \frac{1}{2\pi^2\hbar^3}\left[\int_0^{p_0} f_{FD}(p, \boldsymbol{r})\chi(p, \boldsymbol{r}) p^2 dp + \int_{p_0}^{\infty} f_{FD}(p, \boldsymbol{r}) p^2 dp\right]. \quad (16)$$

Here, $f_{FD}(\boldsymbol{p}, \boldsymbol{r})$ is the Fermi-Dirac distribution function, and the momentum $p_0 = \sqrt{2m_e e\Phi(\boldsymbol{r})}$ is used to divide

the plasma electrons into free and negative-energy ones as discussed in the body of manuscript. In order to compare with classical molecular dynamics (CMD) simulations presented in the manuscript, here the bare ion is assumed and the degeneracy effect between initial and recombined bound electrons is neglected.

## II. Results of Electron density distribution

In figure 2, the CMD results of electron density deviations $\delta\rho(r)$ are compared with those of Fermi-Dirac distribution and the present model with $\rho_e = 10^9/cm^3; \mathrm{T_e} = 5.5\mathrm{K}, \Gamma_e = 0.49$ and $\mathrm{T_e} = 11.5\mathrm{K}, \Gamma_e = 0.23$, respectively. In this case, thus the lines of $\delta\rho(r)$ from Eq. (13) and (14) are coincided. It can be found that there are very good agreements between the present model and CMD results, but deviating obviously from the Fermi-Dirac results. In the present model, the free-electron distribution is same with Fermi-Dirac distribution, which also agree well with the CMD free-electron density distributions, as shown in figure 2. Here, $p_0 = \sqrt{2m_e e\Phi_{\mathrm{DH}}(\boldsymbol{r})}$ is approximated with Debye-Hückel potential $\Phi_{\mathrm{DH}}(\boldsymbol{r})$. These results indicate that the difference between full Fermi-Dirac distribution and CMD simulation can only come from the different treatments of negative-energy electrons distribution.

The Fermi-Dirac distribution significantly overestimates the plasma-electron densities around the targeted ion, indicating the non-equilibrium feature in this case. As discussed in the body of manuscript, Fermi-Dirac distribution describes the distribution of both free and bound electrons in an equilibrated system consisting of free electrons, ions, and atoms. For the case of UNPs, the dominating particles are the ground-state atoms, whose contribution to Fermi-Dirac distribution leads to the overestimations of the electron distribution around the targeted ion.

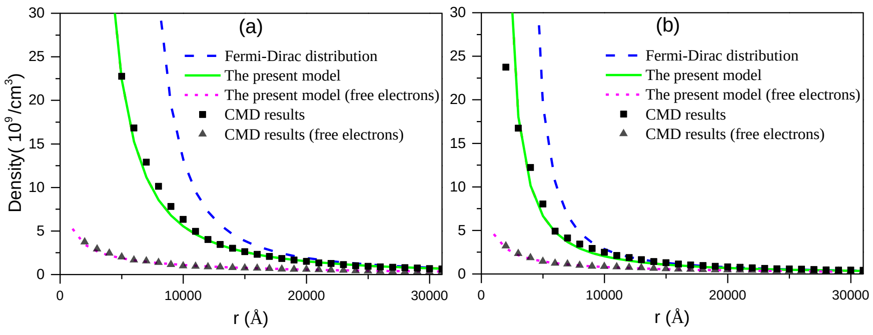


Figure 2 The electron density fluctuation $\delta\rho(r)$ around an ion (Q=1, at origin) embedded in the UNPs with (a) $\rho_e = 10^9/\mathrm{cm}^3, \mathrm{T_e} = 5.5\mathrm{K}$ and (b) $\rho_0 = 10^9/\mathrm{cm}^3, \mathrm{T_e} = 11.5\mathrm{K}$.

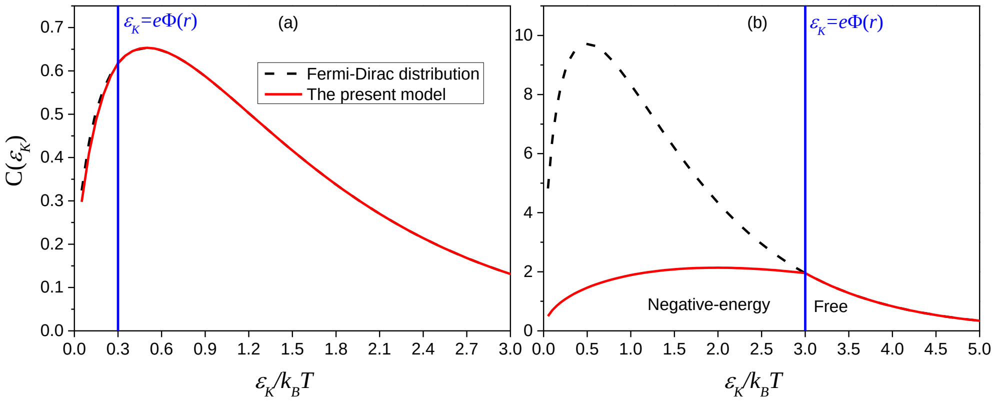


Figure 3 The kinetic-energy distribution of plasma-electron density at positions with (a) $e\Phi(\boldsymbol{r}) = 0.3k_BT$ and (b) $e\Phi(r) = 3k_BT$.

In order to gain deeper insight into the effect of negative-energy electrons on total electron density, a distribution factor $C(\varepsilon_K)$ is defined to meet with

$$\rho(\boldsymbol{r}) = \rho_0 \int_0^\infty C(\varepsilon_K) d\varepsilon_K = \frac{1}{2\pi^2\hbar^3}\left[\int_0^{p_0} f_{FD}(p,\boldsymbol{r})\chi(p,\boldsymbol{r})p^2dp + \int_{p_0}^\infty f_{FD}(p,\boldsymbol{r})p^2dp\right], \quad (17)$$

and

$$C(\varepsilon_K) = \begin{cases} \dfrac{f_{FD}(p,\boldsymbol{r})\chi(p,\boldsymbol{r})p}{4\pi^2\hbar^3\rho_0}, (p < p_0) \\ \dfrac{f_{FD}(p,\boldsymbol{r})p}{4\pi^2\hbar^3\rho_0}, (p \geq p_0) \end{cases}, \quad (18)$$

where $\varepsilon_K = p^2/(2m_e)$ is the kinetic energy of electrons.

Using equation (18), the kinetic-energy dependence of $C(\varepsilon_k)$ can be computed for position $\boldsymbol{r}$. For a plasma with temperature $T$, the $C(\varepsilon_k)$ for the conditions of $e\Phi(\boldsymbol{r}) = 0.3k_BT$ and $3k_BT$ are obtained and compared with the ones of Fermi-Dirac distribution, as shown in figure 3 (a) and (b). It can be found that the free-electron distribution dominates the total electron density when $e\Phi(\boldsymbol{r}) < k_BT$, and the discrepancy of distribution between different treatments of negative-energy electrons is negligible, as shown in figure 3 (a). But the negative-energy electron distribution becomes important in the case of $e\Phi(\boldsymbol{r}) > k_BT$, as shown in figure 3 (b). It should be noted that the integration of $C(\varepsilon_k)$ on $\varepsilon_k$ is the electron density. Therefore, the different treatments of negative-energy electron distribution would lead to large difference of the plasma-electron density obtained, especially for the cases of moderately/strongly coupled plasmas.
